# Supplementary material for: Graph-Induced Rank Structures and their Representations
Source: arXiv:1911.05858 source file (2021-06-26)
Supplement: Supplementary file 1 [file quadratureformula.tex]

\section{Convergence of quadrature formula for log kernel} \label{appendix:quadraturelog}

If the solution $\sigma$ is sufficiently smooth, it is easy to show that
\begin{displaymath}
 \left| \int^{2\pi}_{0}  \log(2 - 2\cos(\theta-\varphi)) \sigma(\varphi) d\varphi - \sum_{k=0, k\ne l}^{n-1} w_{l,k} \log (2 - 2\cos(\theta_l-\varphi_k))  \sigma (\varphi_{k}) \right| \leq \frac{K}{n^2}
\end{displaymath}
To see this, it is sufficient to analyze the convergence rate for $\theta=0$, i.e.  
$$ I =  \int^{2\pi}_0 \log (2 - 2\cos(\varphi))  \sigma(\varphi) d\varphi  $$
Denote $h=\tfrac{2\pi}{n}$ and approximate $I$ by:
\begin{multline}
    I_{n} =  h  (1+\alpha) \log (2 - 2\cos(\varphi_1))  \sigma(\varphi_{1}) +   h \sum^{n-2}_{k=2} \log (2 - 2\cos(\varphi_k)) \sigma(\varphi_{k}) \\
+ h  (1+\beta) \log (2 - 2\cos(\varphi_{n-1}))  \sigma(\varphi_{n-1})
\end{multline}
where $\alpha$ and $\beta$ are correction parameters which must be appropriately chosen. Exploiting periodicity, notice that:
\begin{multline*} |I - I_{n}| \leq   \frac{K_1}{n^2} + \left| \int^{ \tfrac{2\pi}{n} }_{ -\tfrac{2\pi}{n} } \log (2 - 2\cos(\varphi)) \sigma(\varphi) d\varphi    - \right. \\
\left. h  (\tfrac{1}{2}+\alpha) \log(2 - 2\cos(\varphi_1))  \sigma(\varphi_{1}) -  h  (\tfrac{1}{2}+\beta) \log(2 - 2\cos(-\varphi_{1}))  \sigma(-\varphi_{1})    \right|
\end{multline*}
Expanding $\sigma(\varphi)$ in a Taylor series around the origin:
$$ \sigma(\varphi) =   \sigma(0) +  \sigma{'}(0) \varphi  + \frac{\sigma{''}(\xi(\varphi ))}{2} \varphi^{2}  $$
and with some further shenanigans, we obtain:
\begin{eqnarray*}
|I - I_{n}| & \leq &  \frac{K_1}{n^2} +  \frac{K_2}{n^2} + \left|  \sigma(0) \left(  \int^{ \tfrac{2\pi}{n} }_{ - \tfrac{2\pi}{n} } \log  (2 - 2\cos(\varphi))  d \varphi - \right. \right. \\  
& & \left.\left.  h  ( \tfrac{1}{2} +\alpha) \log (2 - 2\cos(\varphi_1))  -  h  (\tfrac{1}{2}+\beta) \log (2 - 2\cos(\varphi_{1}))   \right)  \right|  + \\ 
&  & \left|  \sigma'(0) \left(  \int^{ \tfrac{2\pi}{n} }_{ - \tfrac{2\pi}{n} } \varphi \log  (2 - 2\cos(\varphi))  d \varphi -  h  ( \tfrac{1}{2} +\alpha) \varphi_1\log (2 - 2\cos(\varphi_1))  +\right. \right. \\  
& & \left.\left.   h  (\tfrac{1}{2}+\beta)\varphi_1 \log (2 - 2\cos(\varphi_{1}))   \right)  \right|  \\
& = &  \frac{K_1}{n^2} +  \frac{K_2}{n^2} + \left|  \sigma(0) \left( 2 \int^{ \tfrac{2\pi}{n} }_{0 } \log  (2 - 2\cos(\varphi))  d \varphi - h  \log (2 - 2\cos(\varphi_1)) \right. \right. \\  
& & \left.\left. - h  \alpha\log (2 - 2\cos(\varphi_1))  -  h  \beta \log (2 - 2\cos(\varphi_{1}))   \right)  \right|  + \\ 
&  & \left|  \sigma'(0) \left( 0  -  h  \alpha \varphi_1\log (2 - 2\cos(\varphi_1))  +   h  \beta\varphi_1 \log (2 - 2\cos(\varphi_{1}))   \right)  \right|  
\end{eqnarray*}
The last two terms in the above inequality can be set to zero by selecting:
$$ \alpha = \beta = \frac{ \int^{ \tfrac{2\pi}{n} }_{0 } \log  (2 - 2\cos(\varphi))  d \varphi   }{ \tfrac{2\pi}{n} \log  (2 - 2\cos\left(\tfrac{2\pi}{n})\right)    } - \tfrac{1}{2} $$
yielding an $\mathcal{O}(n^{-2}) $ method overall.
