# Supplementary material for: Graph-Induced Rank Structures and their Representations
Source: arXiv:1911.05858 source file (2021-06-26)
Supplement: Supplementary file 2 [file EDVexample.tex]

\section{Examples of an EDV representation}

Construction algorithm for more complicated flows. For example:
\begin{eqnarray*}
	g_1 & = & V^T_1 x_1 \\
	g_2 & = & V^T_2 x_2 + W_{2-1} g_1 \\
	g_3 & = & V^T_3 x_3 + W_{3-2} g_2 \\
	g_4 & = & V^T_4 x_4 + W_{4-3} g_3  + W_{4-1} g_1 \\
	g_5 & = & V^T_5 x_5 + W_{5-4} g_4    \\
	g_6 & = & V^T_6 x_6  +  W_{6-5} g_5 + W_{6-3} g_3   
\end{eqnarray*}
$$
\begin{array}{lclclclclclcl}
b_1 & = & D_1 x_1 &                            \\
b_2 & = & D_2 x_2 & + & U_{2-1} g_1 &                \\
b_3 & = & D_3 x_3 &+ & U_{3-2} g_2                        \\
b_4 & = & D_4 x_4 & + & U_{4-3} g_3 &                      \\
b_5 & = & D_5 x_5 & + & U_{5-4} g_4 & + &   U_{5-2} g_2                                  \\  
b_6 & = & D_6 x_6 & + & U_{6-5} g_5 & + & U_{6-1} g_1    
\end{array}  
$$
yields: \\
\resizebox{1.1\textwidth}{!}{
		$
	\begin{bmatrix}
	\mathbf{D_1} &  &  & &  &  \\
	  U_{2-1} V^T_1  & \mathbf{D_2} &  &  &  &  \\
	   U_{3-2} W_{2-1} V^T_1  &    U_{3-2} V^T_2  & \mathbf{D_3} &  & &  \\
	   U_{4-3}  W_{3-2}  W_{2-1} V^T_1 &  U_{4-3} W_{3-2}   V^T_2     &   U_{4-3} V^T_3   & \mathbf{D_4} & &   \\
	 \left( U_{5-4}  W_{4-3}  W_{3-2}  +U_{5-2} \right)  W_{2-1} V^T_1    &   \left(U_{5-4} W_{4-3} W_{3-2}   + U_{5-2} \right)V^T_2   &   U_{5-4} W_{4-3}  V^T_3    &   U_{5-4} V^T_4  & \mathbf{D_5} &\\
	   U_{6-5} (  ( W_{5-4}  W_{4-3}  W_{3-2} + W_{5-2})W_{2-1} +  U_{6-1}) V^T_1   &   U_{6-5} \left( W_{5-4} W_{4-3} W_{3-2} +  W_{5-2}\right)  V^T_2     &   U_{6-5} W_{5-4} W_{4-3}   V^T_3     &   U_{6-5} W_{5-4} V^T_4    &  U_{6-5} V^T_5    & \mathbf{D_6}
	\end{bmatrix}$ }
	A permutation of the entries gives: \\
\resizebox{1.1\textwidth}{!}{
	$
	\begin{bmatrix}
   \begin{bmatrix}  \mathbf{D_1} & 0 \\ U_{6-5} (  ( W_{5-4}  W_{4-3}  W_{3-2} + W_{5-2})W_{2-1} +  U_{6-1}) V^T_1 & \mathbf{D_6} \end{bmatrix} &    \begin{bmatrix}0  & 0 \\U_{6-5} \left( W_{5-4} W_{4-3} W_{3-2} +  W_{5-2}\right)  V^T_2  & U_{6-5} V^T_5 \end{bmatrix}   &    \begin{bmatrix} 0 & 0\\ U_{6-5} W_{5-4} W_{4-3}   V^T_3    & U_{6-5} W_{5-4} V^T_4  \end{bmatrix}  \\
   \begin{bmatrix}  U_{2-1} V^T_1   & 0 \\ \left( U_{5-4}  W_{4-3}  W_{3-2}  +U_{5-2} \right)  W_{2-1} V^T_1 & 0 \end{bmatrix} &    \begin{bmatrix}\mathbf{D_2} & 0 \\ \left(U_{5-4} W_{4-3} W_{3-2}   + U_{5-2} \right)V^T_2  & \mathbf{D_5} \end{bmatrix}   &    \begin{bmatrix} 0 & 0 \\ U_{5-4} W_{4-3}  V^T_3 & U_{5-4} V^T_4  \end{bmatrix}  \\
   \begin{bmatrix}U_{3-2} W_{2-1} V^T_1 & 0 \\ U_{4-3}  W_{3-2}  W_{2-1} V^T_1  &  0 \end{bmatrix} &    \begin{bmatrix} U_{3-2} V^T_2   & 0 \\ U_{4-3} W_{3-2}   V^T_2   & 0 \end{bmatrix}    &   \begin{bmatrix} \mathbf{D_3} & 0 \\ U_{4-3} V^T_3  & \mathbf{D_4} \end{bmatrix} 
	\end{bmatrix}$  }
